# Supplementary material for: Search for the decay $B^0\to\phi\mu^+\mu^-$
Source: arXiv:2201.10167 source file (2022-05-13)
Supplement: Supplementary file 1 [file appendix.tex]

% ===============================================================================
% Purpose: appendix to the standard template: standard symbol alises from Ulrik
% Author: Tomasz Skwarnicki
% Created on: 2009-09-24
% ===============================================================================

%{\noindent\normalfont\bfseries\Large Appendices}
\section*{Appendices}

\appendix

\section{Standard References}
\label{sec:StandardReferences}
Below is a list of common references, as
well as a list of all \lhcb publications.
As they are already in prepared bib files, they can be used as simply as
\texttt{\textbackslash cite\{LHCb-DP-2008-001\}} to get the \lhcb detector paper.
The references are defined in the files \texttt{main.bib},  \texttt{LHCb-PAPER.bib},
\texttt{LHCb-CONF.bib}, \texttt{LHCb-DP.bib} \texttt{LHCb-TDR.bib} files, with obvious contents.
Each of these have their \texttt{LHCb-ZZZ-20XX-0YY} number as their cite code.
If you believe there is a problem with the formatting or
content of one of the entries, then get in contact with the Editorial
Board rather than just editing it in your local file,
since you are likely to need the latest version just before submitting the article.

%%%%%%%%%%%%%%%%%%%%%%%%%%%%%%%%%%
\newcommand{\showcite}[1]{\texttt{#1}~\cite{#1}}%
\newcommand{\revshowcite}[1]{\begin{minipage}{1cm}\cite{#1}\end{minipage}\texttt{#1}}%
%%%%%%%%%%%%%%%%%%%%%%%%%%%%%%%%%%
\begin{center}
  % [inline block 0: 5 envs, 37623 chars -> data_tex | \begin{longtable}{ll} \caption{\small Standard references.}\label{tab:Refs}...]

\end{center}}

\section{Standard symbols}

As explained in Sect.~\ref{sec:typography} this appendix contains standard
typesetting of symbols, particle names, units etc.\ in \lhcb
documents.

In the file \texttt{lhcb-symbols-def.tex}, which is included, a
large number of symbols is defined. While they can lead to quicker
typing, the main reason is to ensure a uniform notation within a
document and between different \lhcb documents. If a symbol
like \texttt{\textbackslash CP} to typeset \CP violation is available
for a unit, particle name, process or whatever, it should be used.  If
you do not agree with the notation you should ask to get the
definition in \texttt{lhcb-symbols-def.tex} changed rather than just
ignoring it.

All the main particles have been given symbols. The \B mesons are thus
named \Bp, \Bd, \Bs, and \Bc. There is no need to go into math mode to
use particle names, thus saving the typing of many \$ signs. By
default particle names are typeset in italic type to agree with the
PDG preference. To get roman particle
names you can just change
\texttt{\textbackslash setboolean\{uprightparticles\}\{false\}}
to \texttt{true} at the top of this template.

There is a large number of units typeset that ensures the correct use
of fonts, capitals and spacing. As an example we have
$\mBs=5366.3\pm0.6\mevcc$. Note that \mum is typeset with an upright
$\upmu$, even if the particle names have slanted Greek letters.

A set of useful symbols are defined for working groups. More of these
symbols can be included later. As an example in the Rare Decay group
we have several different analyses looking for a measurement of
\Cpeff7 and \Opep7.

% This is an automatically generated appendix to template.tex. 
% When included it will show all the symbols defined in lhcb-symbols-def.tex.
%
% To regenerate with the latest definitions run the script python listsymbols.py

\section{List of all symbols}
\label{sec:listofsymbols}
\subsection{Experiments}
% [inline block 1: 45 envs, 37654 chars -> data_tex | \begin{tabular*}{\linewidth}{@{\extracolsep{\fill}}l@{\extracolsep{0.5cm}}l@{\extracolsep{\fill}}l@{\extracolsep{0.5cm}}...]
